# Supplementary material for: Microwave-free vector magnetometry with nitrogen-vacancy centers along a single axis in diamond
Source: arXiv:1904.04361 source file (2020-04-14)
Supplement: Supplementary file 1 [file 20190408_microwave_free_vector_magnetometry_using_nitrogen_vacancy_centers_in_diamond--supplementary.pdf]

# Microwave-free vector magnetometry with nitrogen-vacancy centers along a single axis in diamond

Huijie Zheng<sup>1\*</sup>, Zhiyin Sun<sup>2,3\*</sup>, Georgios Chatzidrosos<sup>1</sup>, Chen Zhang<sup>4</sup>, Kazuo Nakamura<sup>5</sup>, Hitoshi Sumiya<sup>6</sup>, Takeshi Ohshima<sup>7</sup>, Junichi Isoya<sup>8</sup>, Jörg Wrachtrup<sup>4</sup>, Arne Wickenbrock<sup>1,2</sup> & Dmitry Budker<sup>1,2,9,10</sup>

<sup>1</sup>*Johannes Gutenberg-University Mainz, 55128 Mainz, Germany*

<sup>2</sup>*Helmholtz-Institute Mainz, 55099 Mainz, Germany*

<sup>3</sup>*Laboratory for Space Environment and Physical Sciences, Harbin Institute of Technology, 150001 Harbin, China*

<sup>4</sup>*Institute of Physics, University of Stuttgart and Institute for Quantum Science and Technology IQST, 70174 Stuttgart, Germany*

<sup>5</sup>*Application Technology Research Institute, Tokyo Gas Company, Ltd., Yokohama, 230-0045 Japan*

<sup>6</sup>*Advanced Materials Laboratory, Sumitomo Electric Industries, Ltd., Itami, 664-0016 Japan*

<sup>7</sup>*Takasaki Advanced Radiation Research Institute, National Institutes for Quantum and Radiological Science and Technology, Takasaki, 370-1292, Japan*

<sup>8</sup>*Faculty of Pure and Applied Sciences, University of Tsukuba, Tsukuba, 305-8573 Japan*

<sup>9</sup>*Department of Physics, University of California at Berkeley, California 94720-7300, USA*

<sup>10</sup>*Nuclear Science Division, Lawrence Berkeley National Laboratory, Berkeley, CA 94720, USA*

## 1 Supplementary Information

**Illustration of the working principle of the transverse field detection.** The PL-GSLAC feature changes its shape according to the applied transverse field, which, however, does not depend on the direction of the field in the  $x$ - $y$  plane. We approximate the PL-GSLAC feature as a function of transverse field by a 2D Lorentzian function symmetric around the  $z$ -axis, indicated in Fig. S1 (a) (i). The maximum PL signal corresponds to zero transverse magnetic field and it decreases as

the magnitude of the transverse field increases. When applying a transverse magnetic field rotating around the  $z$ -axis, the PL signal is reduced but remains constant (no oscillating component) in the absence of a transverse DC field, indicated by the red curve in Fig. S1 (a) (ii). In the presence of a transverse field, the PL signal is off center from the coordinate origin and shows a minimum value when the rotating field reaches the same direction as the transverse field being interrogated, shown in Fig. S1 (a) (iii), (iv) and (v). The difference between the PL signals with (red curve) and without (blue curve) applied transverse field is shown in Fig. S1 (b). This is then demodulated by a LIA which delivers the information of both the amplitude and the angle of the magnetic field to be measured, as shown in Fig. S1 (c).

The  $x$  and  $y$  axes can be calibrated by tuning the reference phase of the modulation field. In our case, the measured  $x$  and  $y$  axes are set along the  $x$ - and  $y$ -modulating Helmholtz coils. The reference phase of the LIA was set so that a magnetic field along the  $x$ -axis corresponds to phase zero (and negative amplitude). The LIA output shows a maximum value at  $0^\circ$  when applying a field along  $x$ -axis, shown in Fig. S1 (c). An applied field in any other direction leads to an oscillating PL signal with a corresponding phase. Therefore, the phase output of the LIA is the angle between the transverse field to be measured and the defined  $x$  and  $y$  axes.

The modulation field is generated with two Helmholtz coils excited by two sine waves with the same frequency but  $90^\circ$ -shifted phases, with an amplitude of  $\approx 20 \mu\text{T}$ . The phase between these two modulating fields as well as the amplitudes are adjusted to get minimal magnitude output of the LIA without transverse field.

**Demonstration of an  $x$ - $z$  measurement.** Full vector measurements of magnetic fields require a measurement in the  $z$  direction. They are carried out by applying an additional modulated field along  $z$  with a different frequency (than in the transverse direction) and demodulation of the PL signal. A matrix of 2D vector magnetic fields in  $x$ - $z$  plane was measured to demonstrate the method with various  $B_x$  and  $B_z$  in the range of  $\pm 3 \mu\text{T}$ . The angle of the field can be calculated as  $\arctan(B_z/B_x)$  from the applied currents and calibration factors of the two coils. Figure S2

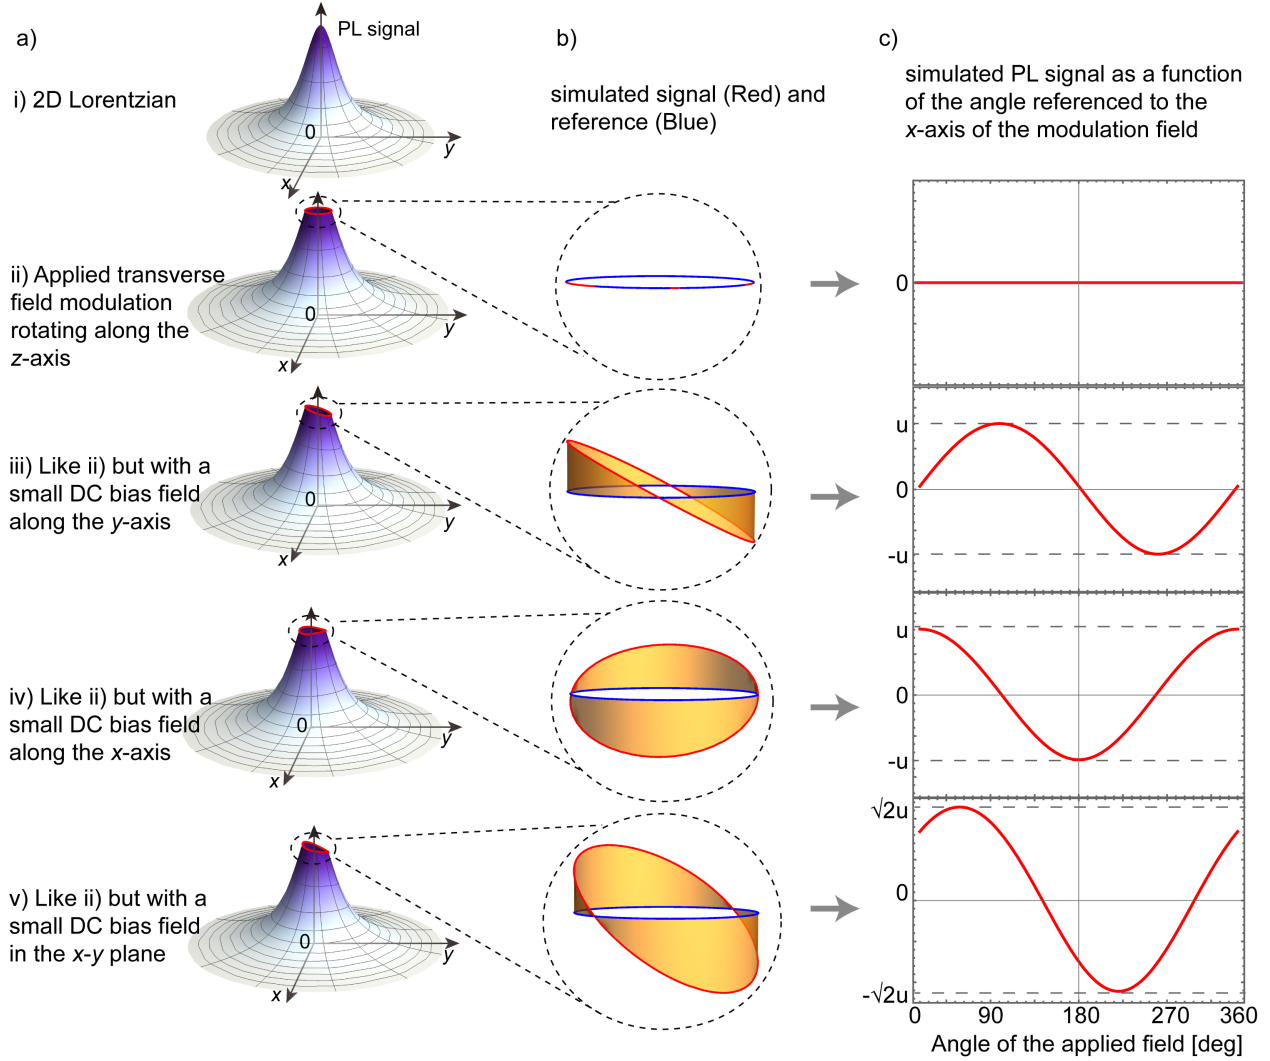

Figure S1: (a) Simulated PL signals as a function of transverse field. The red curves are the trajectories of PL signals superimposed on the 2D Lorentzian contrast function. Figures i) to v), correspond to different show cases: i) no modulated fields and no bias fields, ii) with modulated fields but no bias fields (the time-averaged PL drops), iii) with modulated fields and bias field along  $y$ , iv) with modulated fields and bias field along  $x$ , v) with modulated fields and bias field in  $x$ - $y$  plane, respectively. (b) The simulated PL signals with modulating magnetic field in the presence/absence (red curve/blue curve) of a bias field. (c) Simulated PL signals [in the same coordinate system as in column (a)] as a function of the angle of the modulated field referenced to the  $-x$ -axis for transverse fields corresponding to (a) and (b).

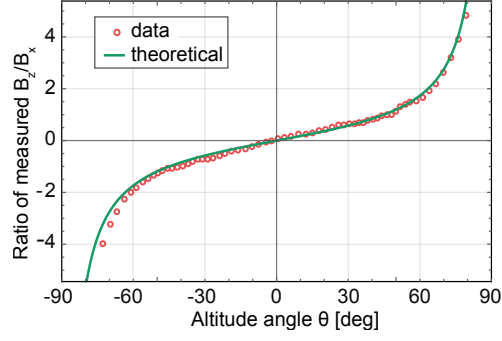

Figure S2: The ratios of measured fields  $B_z/B_x$  corresponding to different angles are calculated from the applied fields in  $x$ - $z$  plane. The solid green line shows an arctangent dependence.

shows that the ratios of the measured fields  $B_z$  and  $B_x$  correspond to different angles following the expected arctangent curve. The comparison corroborates the method's effectiveness.
